# Supplementary material for: CSP4SDG: Constraint and Information-Theory Based Role Identification in Social Deduction Games with LLM-Enhanced Inference
Source: arXiv:2511.06175 source file (2025-11-09)
Supplement: Supplementary file 1 [file aaai2026-supp.tex]

%File: aaai2026-unified-supp.tex
%
% UNIFIED AAAI 2026 SUPPLEMENTARY MATERIAL TEMPLATE
% To switch between anonymous submission and camera-ready versions,
% simply change the next line:
%
% For ANONYMOUS SUBMISSION: uncomment the next line
%\def\aaaianonymous{true}
%
% For CAMERA-READY VERSION: comment out or delete the next line
% \def\aaaianonymous{true}
%
%%%%%%%%%%%%%%%%%%%%%%%%%%%%%%%%%%%%%%%%%%%%%%%%%%%%%%%%%%%%%%%%%%%%%%%

\documentclass[letterpaper]{article} % DO NOT CHANGE THIS

% Conditional package loading based on version
\ifdefined\aaaianonymous
    \usepackage[submission]{aaai2026}  % Anonymous submission version
\else
    \usepackage{aaai2026}              % Camera-ready version
\fi

\usepackage{times}  % DO NOT CHANGE THIS
\usepackage{helvet}  % DO NOT CHANGE THIS
\usepackage{courier}  % DO NOT CHANGE THIS
\usepackage[hyphens]{url}  % DO NOT CHANGE THIS
\usepackage{graphicx} % DO NOT CHANGE THIS
\urlstyle{rm} % DO NOT CHANGE THIS
  % DO NOT CHANGE THIS
\usepackage{natbib}  % DO NOT CHANGE THIS AND DO NOT ADD ANY OPTIONS TO IT
\usepackage{caption} % DO NOT CHANGE THIS AND DO NOT ADD ANY OPTIONS TO IT
\frenchspacing  % DO NOT CHANGE THIS
\setlength{\pdfpagewidth}{8.5in} % DO NOT CHANGE THIS
\setlength{\pdfpageheight}{11in} % DO NOT CHANGE THIS

% These are recommended to typeset algorithms but not required.
\usepackage{algorithm}
\usepackage{algorithmic}
\usepackage{amsmath}
\usepackage{booktabs}
\usepackage{subcaption}
\usepackage{siunitx}
\usepackage{comment}
\usepackage{multirow}
\usepackage{amsthm}
\usepackage{amssymb}
\usepackage[utf8]{inputenc}
\DeclareUnicodeCharacter{21D2}{\ensuremath{\Rightarrow}}

\theoremstyle{definition}

% These are recommended to typeset listings but not required.
\usepackage{newfloat}
\usepackage{listings}
\DeclareCaptionStyle{ruled}{labelfont=normalfont,labelsep=colon,strut=off} % DO NOT CHANGE THIS
\lstset{% 
	basicstyle={\footnotesize\ttfamily},
	numbers=left,numberstyle=\footnotesize,xleftmargin=2em,
	aboveskip=0pt,belowskip=0pt,
	showstringspaces=false,tabsize=2,breaklines=true}
\floatstyle{ruled}
\newfloat{listing}{tb}{lst}{}
\floatname{listing}{Listing}

\pdfinfo{
/TemplateVersion (2026.1)
}

\setcounter{secnumdepth}{0} %May be changed to 1 or 2 if section numbers are desired.

% Title - conditionally set based on version
\title{Appendix for ``CSP4SDG: Information-Gain–Weighted Probabilistic Constraint Solving in Social Deduction Games''}

% Author and affiliation information
\ifdefined\aaaianonymous
\author{
    Anonymous Submission
}
\affiliations{
    % Leave affiliations empty for anonymous submission
}
\else
\author{
    Kaijie Xu\textsuperscript{\rm 1},
    Fandi Meng\textsuperscript{\rm 2},
    Clark Verbrugge\textsuperscript{\rm 1},
    Simon Lucas\textsuperscript{\rm 2}\\
}
\affiliations{
    \textsuperscript{\rm 1}Department of Computer Science, McGill University, Montreal, Quebec, Canada\\
    \textsuperscript{\rm 2}Queen Mary University of London, London, United Kingdom\\
    kaijie.xu2@mail.mcgill.ca, f.meng@qmul.ac.uk, clump@cs.mcgill.ca, simon.lucas@qmul.ac.uk
}
\fi

\begin{document}

\maketitle

\begin{abstract}
This document complements the main paper by consolidating all material that could not fit into the body text. \textbf{Appendix~A} surveys prior work on role inference, constraint programming, and information-theoretic reasoning, situating CSP4SDG within the broader literature.   \textbf{Appendix~B} presents the mathematical proofs— including the equivalence between our soft- and hard-assertion formulations—that underpin the framework’s theoretical guarantees.   \textbf{Appendix~C} supplies comprehensive dataset descriptions, the LLM-based constraint-extraction pipeline, pre-processing scripts, and evaluation protocols required for reproducibility.   \textbf{Appendix~D} introduces the detailed hyper parameters and computing infrastructure information of the experiments.  \textbf{Appendix~E} shows the results and interpretation of the statistical significance analysis. \textbf{Appendix~F} details the prompt head we used in the experiments. \textbf{Appendix~G} includes the full results on dialogue dataset on both Truthful-Good condition and Lying-Good condition. \textbf{Appendix~H} presents the full table for the AvalonLogs Dataset results. \textbf{Appendix~I} shows the results of ablation experiments on manual weights combination.
\end{abstract}

% ----------- Supplementary Content Starts Here -----------

\appendix
\input{Appendix/background}
\input{Appendix/proof}
\input{Appendix/dataset}
\input{Appendix/experiments}
\input{Appendix/sig_test}
\input{Appendix/prompt}
\input{Appendix/full_table2}
\input{Appendix/avalonlogs}
\input{Appendix/hyperparameter}

% ----------- Supplementary Content Ends Here -----------

% References and End of Paper
% These lines must be placed at the end of your paper
\bibliography{aaai2026}

\end{document}
